# Supplementary material for: Geostatistical modeling to capture seismic-shaking patterns from earthquake-induced landslides
Source: arXiv:1807.08513 source file (2018-07-23)
Supplement: Supplementary file 1 [file SupplementaryMaterial.pdf]

# Supplementary Material: Geostatistical modeling to capture seismic-shaking patterns from earthquake-induced landslides

Luigi Lombardo[1,2*], Haakon Bakka[1], Hakan Tanyas[3], Cees van Westen[3], P. Martin Mai[2], Raphael Huser[1]

July 19, 2018

**Keywords:** Integrated nested Laplace approximation (INLA), Landslide susceptibility, Landslide intensity, Slope unit, Spatial point pattern, Wenchuan and Lushan earthquakes

[1]King Abdullah University of Science and Technology (KAUST), Computer, Electrical and Mathematical Sciences and Engineering (CEMSE) Division, Thuwal 23955-6900, Saudi Arabia.

[2]King Abdullah University of Science and Technology (KAUST), Physical Sciences and Engineering (PSE) Division, Thuwal 23955-6900, Saudi Arabia.

[3]University Twente, Faculty of Geo-Information Science and Earth Observation (ITC), The Netherlands

# 1 Multicollinearity in the Data

Figures SM1 and SM2 show the Pearson correlation coefficients of all continuous covariates. The seismic parameters all show high linear dependency, both for the Lushan and the Wenchuan datasets.

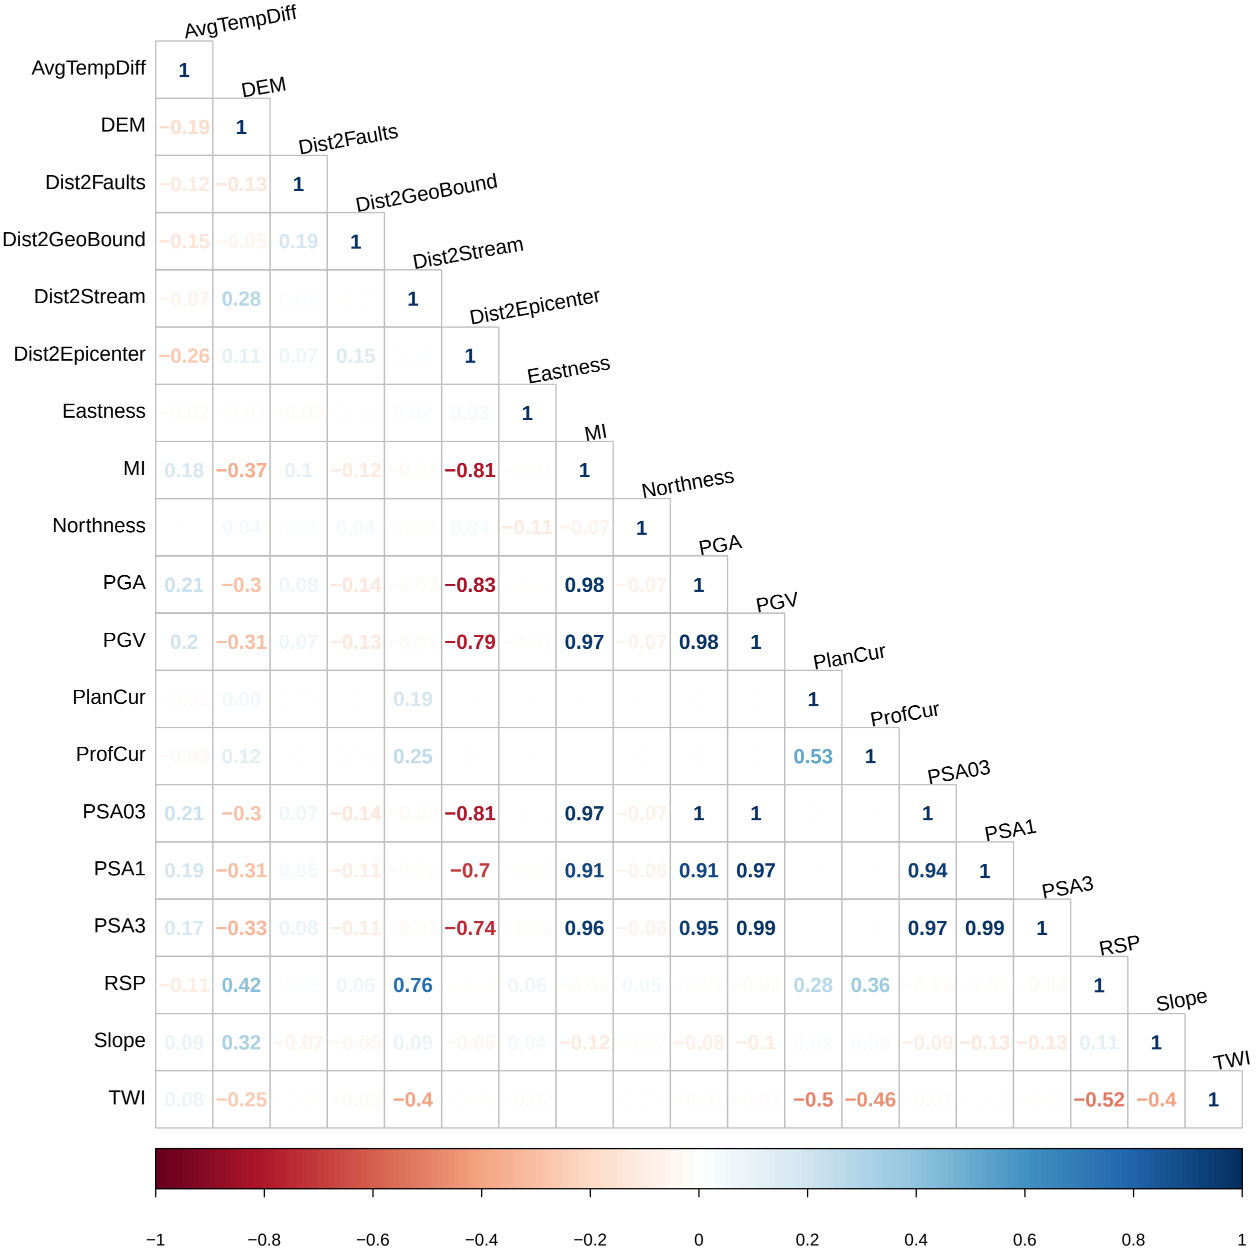


Figure 1: Correlation matrix for covariates in the Lushan dataset.

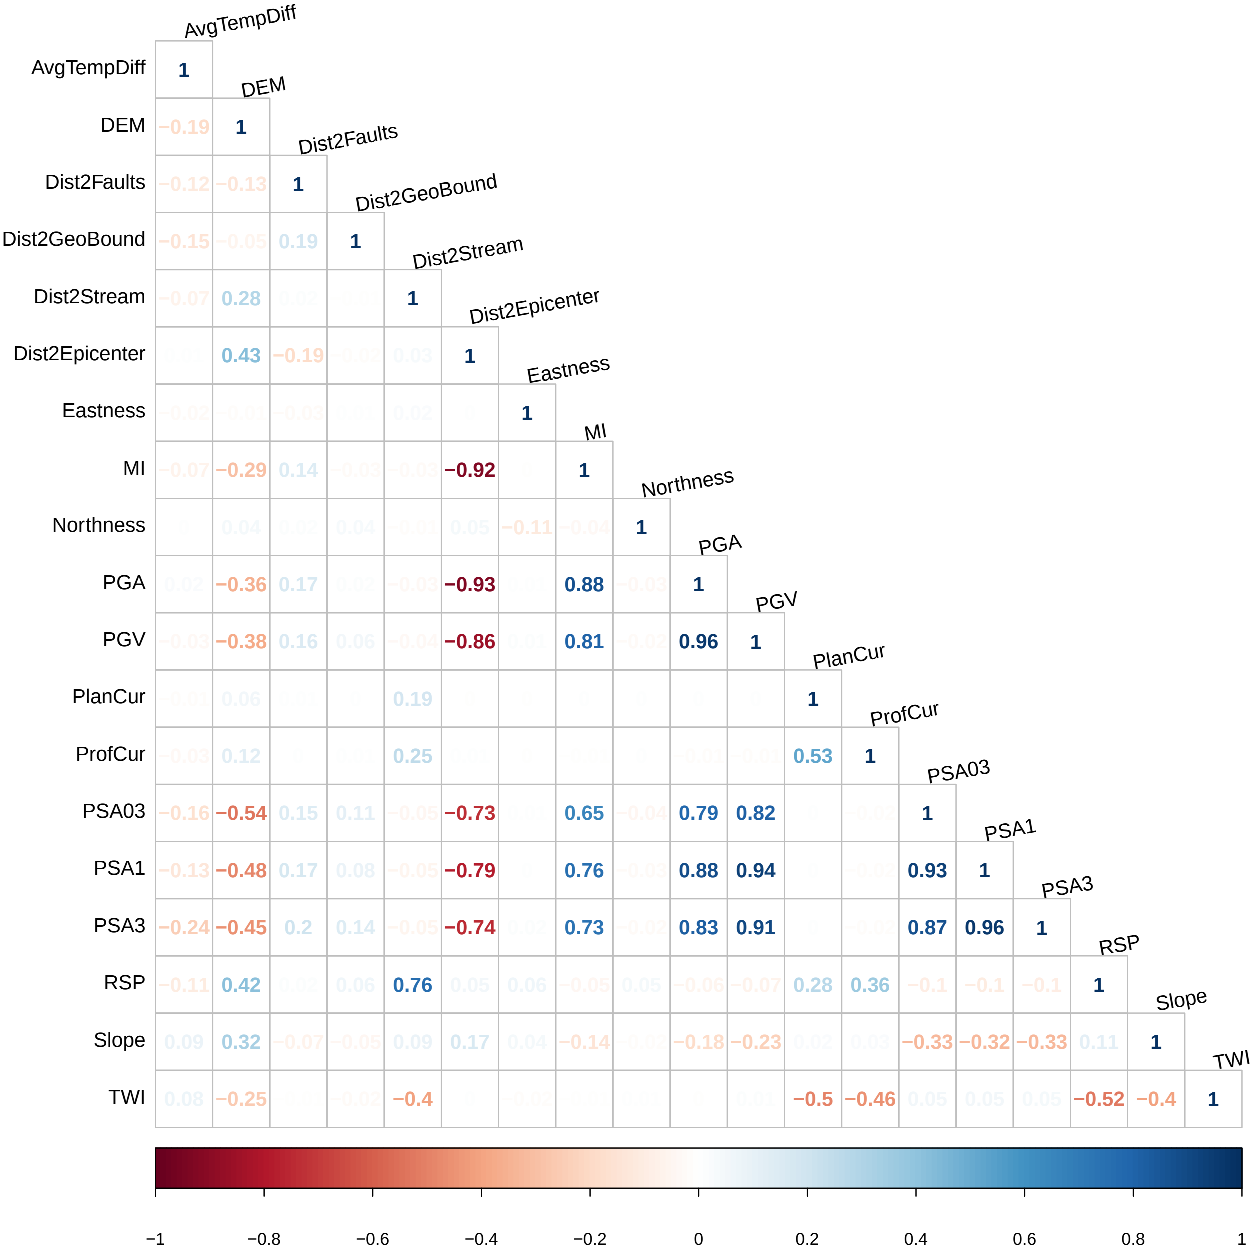


Figure 2: Correlation matrix for covariates in the Wenchuan dataset.

# 2 Interpretation of Covariate Effects

With regard to the interpretation of the results, the geomorphological adequacy of the model is usually inferred from the covariate effects. In this work, we used both fixed (see Figure 8) and random effects (see Figure 10). Some clearly play a dominant role in the model while others were non-significant.

Taking aside the LSE, the second most relevant covariate is the *Slope steepness*, which positively contributes to increase the landslide intensity both for Lushan ($\hat{\beta} = 0.477$) and

Wenchuan ($\hat{\beta} = 0.241$). This is a well-known behavior in the literature (Cama *et al.*, 2015; Donnarumma *et al.*, 2013, e.g.). On two more occasions, covariates appear to play the same role for both earthquakes. *Distance to Geoboundaries* ($\hat{\beta} = -0.099$ for Lushan and $\hat{\beta} = -0.194$ for Wenchuan) decreases the landslide intensity as the distance increases. We interpret this effect as a function of the proximity to geological discontinuities, which can act as favorable sliding planes, especially in the context of adjacent lithotypes with different geotechnical characteristics (see also Castro Camilo *et al.*, 2017). *Eastness* equally contributes to the two models. However, *Eastness* is just one component of the original *Aspect* signal, which is conveniently simplified to a fixed effect in the model. Thus, we present in this paper a comprehensive interpretation of both *Eastness* and *Northness* by recombining their fixed effects into the original *Aspect* scale for clarity. Figure 9 shows our recombined *Aspect* effect, where a positive contribution is marked for east-facing pixels in the Lushan model and east-southeast-facing pixels in the Wenchuan model. The second result agrees well with other contributions. For example, Parker (2013) noted that:

"The aspect of hillslopes also appears to exert a stability control on landslide density, associated with the available heat and magnitude of diurnal heating and cooling cycles, which drive the physical breakdown of exposed bedrock (McFadden *et al.*, 2005; Selby *et al.*, 1982). The occurrence of earthquake-induced landslides on south-facing slopes during the Northridge earthquake (Meunier *et al.*, 2008) and the Wenchuan earthquake (Parker *et al.*, 2010; Chen *et al.*, 2012) has been attributed to this effect. While hillslope materials are highly spatially heterogeneous and anisotropic on smaller spatial scales, data is not currently available to resolve this level of local variability at the regional-scale for landslide inventory analysis".

In addition to heating and cooling cycles, we assume that, the orientation of the hillslope with respect to the ground motion direction of an earthquake should also play an important role.

We interpret the effect of *Elevation* as a possible confounded covariate. From a quick look, *Elevation* appears to contribute positively for Wenchuan ($\hat{\beta} = 0.335$) and negatively for Lushan ($\hat{\beta} = -0.591$). However, we think that this effect is confounded with the actual shaking that took place during the two earthquakes. In fact, the maximum shaking during the Lushan earthquake occurred in the southern sector and across a very extended surface. There, elevation varies quickly across space, including a central, relatively rough lowland where numerous landslides were clustered. For Wenchuan, the maximum shaking within the study area affected a small region with high elevation in the north. For this reason, the landslide scenario only occupied the northern sector with extremely few mass movements at lower elevations. As a result, the model recognizes correlations that are not due to the actual elevation, but rather a result of the coexisting shaking levels.

Other covariates alternatively appear significant for one earthquake or the other. Among these, the *Average Temperature Difference* strongly contributes to the Wenchuan inventory ($\hat{\beta} = 0.308$). We explain the lack of significance for Lushan by the proximity to the epicenter.

The Lushan epicenter is located in the proximity of the study area. Thus, the shaking levels are higher than those of the Wenchuan earthquake (see Figure 2), which occurred almost 100 km away (see Figure 1). For this reason, the earthquake signal is expected to saturate the slope response in the Lushan case, while to generate landslides in the Wenchuan case, the degree of weathering due to temperature changes may have played a determinant role. *Distance to Faults* marks an opposite situation, being significant (and positive, $\hat{\beta} = 0.125$) only for Lushan. This may be due to reduced rock strength and cohesion in the proximity of tectonic alignments, allowing for common erosive processes to remove the source material that feeds landslide initiations. Conversely, at larger distances from the main alignments in the area, the source material may still be in place, thus allowing the earthquake shaking to mobilize it and evolve into a landslide. *Distance to Streams* shows a similar pattern, being significant (and slightly negative, $\hat{\beta} = -0.063$) only for Lushan. This means that as the distance from the streams increases, the estimated landslide count is negatively affected. The same signal is also captured by the *Topographic Wetness Index* and the *Stream Landform* class (both positive). We interpret this as a potential indication of either alluvial deposits along river banks or basal erosion due to water flows, which in turn can give rise to landslides in the presence of strong shaking levels. With a 90 m pixel side, we cover both the river width and part of the river flanks, which may produce this positive effect. It is worth mentioning that by using the centroid to represent the landslide activation, the points may be located more downslope than in reality.

Apart from the LSE, we also consider three more random effects: *Outcropping Lithology*, *Landforms*, and *Land Cover* (see Figure 10). These effects behave very differently in the Lushan and Wenchuan cases. The Wenchuan case, has fewer significant classes; only *Quaternary Clay, Sand, Gravel* is noticeably significant, and positively contributes by increasing the landslide intensity ($\hat{\beta} = 0.174$). This lythotype can be interpreted as a mixed deposit, which in turn may reflect poorer geotechnical properties than more competent rocks outcropping in the area. Surprisingly, none of the *Landforms* play a clear role with the exception of *Open Slopes*, which slightly misses significance while presenting a negative sign ($\hat{\beta} = -0.094$). In terms of *Land Cover*, only *Broadleaved Deciduous Forest* appears to be significant and positive ($\hat{\beta} = 0.752$). The association between this vegetation type and landslides is already known in the literature and, specifically, within the Sichuan province (e.g. Li *et al.*, 2017). However, this relation is typically found in opposite terms. In other words, deciduous forests are usually found to occupy and diversify over mixed landslide deposits. In our case, we also find that landslides occur over this class of land cover. Broadleaved deciduous trees typically lose their leaves during winter and require a very wide but shallow rootage to absorb significant amounts of water and grow back the lost leaves during spring and summer. Therefore, we interpret this correlation in terms of the added weight to slopes, without the additional root strength provided by deep rootages.

For the Lushan earthquake, a greater number of lithologies shows significance. *Devonian Limestone, Dolomite* ($\hat{\beta} = -0.354$), *Permian Sandstone, Limestone* ($\hat{\beta} = -0.316$) and

*Proterozoic Granite* ($\hat{\beta} = -0.166$) all negatively contribute to landslide intensities. This negative contribution can be interpreted as solid rock masses, which are clearly difficult to destabilize, and as lithotypes where seismic amplification does not occur because of low seismic impedance. Similarly, *Silurian Black Shale with Marl, Phyllite, Tuff* presents a negative coefficient ($\hat{\beta} = -0.541$), suggesting the role of seismic propagation in this medium. Shales are characterized by high seismic velocities, despite their natural anisotropy. For instance, Johnston and Christensen (1995), experimentally demonstrated that, even in the case of unfavorable bedding orientation with respect to the wavefield, shales exhibit seismic velocities of approximately 2.0 km/s, which contributes to quickly propagate the earthquake shaking into other more susceptible media.

Positive effects with respect to the Lushan landslide intensity can be recognized in *Jurassic Sandstone, Mudstone* ($\hat{\beta} = 0.360$), *Cretaceous Sandstone, Mudstone, Siltstone* ($\hat{\beta} = 0.443$) and *Quaternary Clay, Sand, Gravel* ($\hat{\beta} = 0.235$). All three represent lithotypes with lower velocity speeds than the other lithological classes. This may indicate greater shaking for a prolonged time, which may produce a higher landslide count.

Ultimately and surprisingly, no *Land Cover* classes showed significance for the Lushan earthquake.

# References


Cama, M., Lombardo, L., Conoscenti, C., Agnesi, V. and Rotigliano, E. (2015) Predicting storm-triggered debris flow events: application to the 2009 Ionian Peloritan disaster (Sicily, Italy). *Nat Hazards Earth Syst Sci* **15**(8), 1785–1806.

Castro Camilo, D., Lombardo, L., Mai, P., Dou, J. and Huser, R. (2017) Handling high predictor dimensionality in slope-unit-based landslide susceptibility models through LASSO-penalized Generalized Linear Model. *Environmental Modelling and Software* **97**, 145–156.

Chen, X.-q., Li, Y., Gao, Q. and Jia, S.-t. (2012) Distribution characteristics of Geo-hazards in Ganxi Valley after the Wenchuan earthquake. *Environmental Earth Sciences* **65**(4), 965–973.

Donnarumma, A., Revellino, P., Grelle, G. and Guadagno, F. M. (2013) *Slope Angle as Indicator Parameter of Landslide Susceptibility in a Geologically Complex Area*, pp. 425–433. Berlin, Heidelberg: Springer.

Johnston, J. E. and Christensen, N. I. (1995) Seismic anisotropy of shales. *Journal of Geophysical Research: Solid Earth* **100**(B4), 5991–6003.

Li, B., Zeng, T., Ran, J., Yue, B., Zhang, M., Shang, T. and Zhu, D. (2017) Characteristics of the early secondary succession after landslides in a broad-leaved deciduous forest in the south Minshan Mountains. *Forest Ecology and Management* **405**, 238–245.

McFadden, L., Eppes, M., Gillespie, A. and Hallet, B. (2005) Physical weathering in arid landscapes due to diurnal variation in the direction of solar heating. *Geological Society of America Bulletin* **117**(1-2), 161–173.

Meunier, P., Hovius, N. and Haines, J. A. (2008) Topographic site effects and the location of earthquake induced landslides. *Earth and Planetary Science Letters* **275**(3), 221–232.

Parker, R. (2013) *Hillslope memory and spatial and temporal distributions of earthquake-induced landslides.* Ph.D. thesis, Durham University.

Parker, R. *et al.* (2010) *Controls on the distribution of landslides triggered by the 2008 Wenchuan earthquake, Sichuan Province, China.* Ph.D. thesis, Durham University.

Selby, M. J. *et al.* (1982) *Hillslope materials and processes.* Oxford University Press.
